# Supplementary material for: Color center fluorescence and spin manipulation in single crystal, pyramidal diamond tips
Source: arXiv:1608.08369 ancillary file (2016-10-28)
Supplement: Supplementary file 1 [file supplementaryfinallrc.pdf]

# Supplementary information for manuscript: Color center fluorescence and spin manipulation in single crystal, pyramidal diamond tips

Richard Nelz,[1] Philipp Fuchs,[1] Oliver Opaluch,[1] Selda Sonusen,[1] Natalia Savenko,[2] Vitali Podgursky,[3] and Elke Neu[1, a)]
[1)] *Universität des Saarlandes, FR 7.2 Experimentalphysik, 66123 Saarbrücken, Germany*
[2)] *Artech Carbon OÜ, Jõe 5, 10151 Tallinn, Estonia*
[3)] *Tallinn University of Technology, Department of Materials Engineering, Ehitajate tee 5, 19086, Tallinn, Estonia*

(Dated: 26 August 2016)

This supplementary material summarizes technical details on the experimental setup. We also present additional photoluminescence (PL) spectra and 3-dimensional PL maps of the diamond tips together with further information on the numerical simulation of photonic properties. The supplementary material also gives further details on the measurement and evaluation of optically detected magnetic resonance (ODMR) spectra and color center lifetimes. Finally, we here summarize details on the plasma treatments as well as the respective electron microscopy images and PL spectra.

## I. EXPERIMENTAL SETUP

We analyze the photoluminescence (PL) of the diamond tips by mounting them onto a three-axes piezoelectric scanner (Attocube ANS xyz100) in our home built confocal microscope. We use a 532 nm DPSS laser (Integrated Optics, Matchbox 532L-21B) and an acousto-optic modulator (AOM, Crystal Technologies, 3200-146, 11 ns rise-time) to realize pulsed and continuous excitation of our samples. A 100× microscope objective (Olympus, LMPLFLN100X) with a numerical aperture (NA) of 0.8 focuses the excitation light onto the sample and collects the PL. Two dichroic mirrors (cut in wavelength: 560 nm) and a dielectric longpass filter (cut in wavelength: 650 nm) separate the excitation light from the emitted PL photons. We subsequently couple the PL to a single mode fiber (Thorlabs SM600, MFD 3.6 - 5.3 $\mu$m, NA 0.1 - 0.14) which serves as a pinhole.

The single mode fiber directs the PL of the sample to our detection setup. This detection setup contains a Hanbury-Brown Twiss interferometer (HBT) consisting of two avalanche photodiodes (APD, Excelitas SPCM-AQRH-14) to obtain the time resolved PL rate of the defects and a grating spectrometer from Princeton Instruments (Acton SpectraPro SP-2500 with Pixis 256OE CCD) to measure the spectral properties of the PL. Using microwave electronics (SpinCore PulseBlaserESR-PRO, Stanford Research Systems SG384, MiniCircuits ZASWA-2-50DR+) together with a moveable nearfield antenna,[1] we are able to perform optically detected magnetic resonance (ODMR) measurements of nitrogen-vacancy (NV) centers as well as coherent manipulation of NV electronic spins.

To quantify the color centers' excited state lifetime, we perform pulsed excitation using a supercontinuum laser (NKT Photonics, EXW-12, pulse length ≈ 50 ps) with a filter system (Varia) to select a defined wavelength range. Together with a time tagging module (PicoQuant, PicoHarp 300), this allows for time correlated (single) photon counting with high temporal resolution.

## II. 3-DIMENSIONAL PL MAPPING AND SPECTRA

Figure S1 summarizes 3-dimensional PL mapping of the tips and is obtained via the following method: First, we measure the PL on each point in the xy-plane. Subsequently, we change the focus to a different z-position of the pyramid and repeat the measurement. Thus, we construct a 3-dimensional PL map. Together with the PL spectra at each z-position, we deduce information about the density of color centers at the respective positions in the pyramid. For the interpretation of the spectra, see the main manuscript.

In the lower row of Fig. S1, a bright background emission is visible in a distance of about 2 $\mu$m to the pyramid base. This background probably results from a contamination on the Si cantilever and is thus not related to the diamond device itself. The epoxy used for gluing the tips to the cantilever only produces minor, broadband PL observed when focusing the laser to the base of the diamond pyramid.

## III. PL SIMULATIONS

To simulate the color centers' emission characteristics inside the pyramidal tip, we use a commercial Finite Difference Time Domain (FDTD) software (Lumerical FDTD Solutions). The software allows for broadband simulations, nevertheless we restrict our analysis to a single wavelength of 700 nm, which corresponds to the center of the used filter window for NV sideband detection. The pyramidal tip is abstracted as a frustum with a square

[a)] Electronic mail: elkeneu@physik.uni-saarland.de

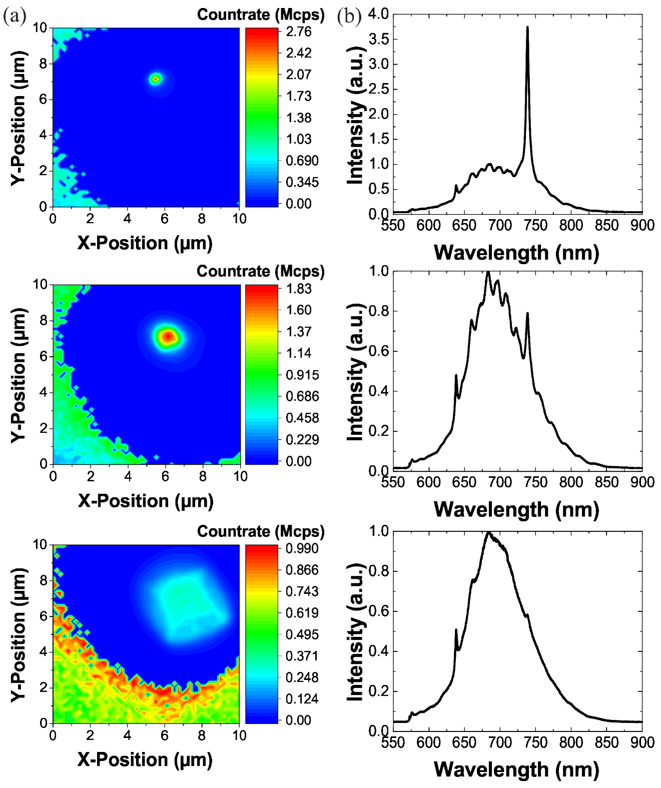


FIG. S1. Mapping of NV fluorescence (680-720 nm) (a) and PL spectra (b) at the bottom (lower), the middle (middle) and the apex (upper) of the tip. The SiV PL is rapidly decreasing compared to the NV PL. Note that the countrates are measured through an OD1 neutral density filter. The spectra are normalized on the maximum in NV PL.

base of $5 \times 5\,\mu\mathrm{m}^2$ that narrows to $20 \times 20\,\mathrm{nm}^2$ at the top, a height of $10\,\mu$m and a refractive index of $n = 2.4$. An electric point dipole, placed in the horizontal center of the pyramid, represents the color center. Its vertical position is varied over the height of the pyramid, corresponding to an experimental excitation in different focal planes (z-positions). The whole simulation area is surrounded by perfectly matched layers and is meshed with $15 \times 15 \times 15\,\mathrm{nm}^3$ Yee cells. A monitor, placed 100 nm above the pyramid's top, records the fields emitted towards the upper half-space. This allows us to calculate the far field and thereby the power radiated into a specific NA.

As sensing applications often demand to maximize the photon flux into the detection optics, our figure of merit is the ratio of the radiated power into a specific NA to the radiated power in homogeneous diamond, here called collection factor $\xi$.

$$\xi = \frac{P_{\mathrm{NA}}}{P_{\mathrm{hom}}} \tag{1}$$

Note that the denominator $P_{\mathrm{hom}} = n \cdot P_0$, with $P_0$ the total time-average power radiated by an electric dipole in vacuum, is independent from the dipole's position inside the diamond. The refractive index $n = 2.4$ is determined by the host material. Thus, the collection factor quantifies the power or the photon flux, respectively, into the NA in a more handy and comparable way than absolute powers do. Note that a high collection efficiency, usually defined with the denominator being the total time-average power radiated by the dipole in the specific dielectric environment, does not necessarily indicate a high photon flux.

## IV. SATURATION

Figure S2 shows the saturation measurement done at the apex of the pyramid detecting PL in the wavelength range from 680 to 720 nm. This detection window has been chosen to separate the NV PL from the SiV PL. We find a saturation power $P_{\mathrm{sat}} = 377(6)\,\mu$W and a maximal countrate $I_\infty = 5.52(3)$ Mcps. The data are fitted with

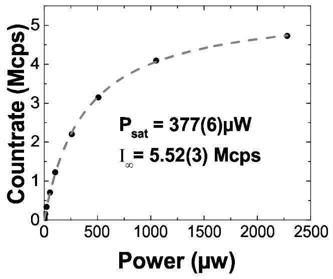


FIG. S2. Saturation measurement at the apex fitted with Eq. 2.

the following function of the excitation power $P$ including a linearly increasing background PL $B$:

$$I(P) = I_\infty \cdot \frac{P}{P + P_{\mathrm{Sat}}} + B \cdot P \tag{2}$$

With this, we calculate an estimation of the PL countrate emitted into the first lens of our confocal microscope. First, we estimate the fraction of the whole NV spectral intensity we detect to be roughly one third of the full intensity. Knowing the transmission of our confocal setup ($T = 44\,\%$) and the detection efficiency of our avalanche photodiodes (70 %) as well as the transmission of the OD1 filter, we estimate the countrate emitted into the first lens to be 500 Mcps. This is easily measurable with a common commercial photodiode as this corresponds to PL in the 100 pW regime.

## V. LIFETIME MEASUREMENTS

We measure the excited state lifetimes of NV $\tau_{\mathrm{NV}}$ and SiV (silicon-vacancy) $\tau_{\mathrm{SiV}}$ along the z-axis of the pyramid. By choosing suitable filters (680 - 720 nm for NV and 735 - 745 nm for SiV), we aim at separating the PL of NV and SiV centers. Fitting the NV PL decay with a

single exponential decay yields very good agreement with the measured data [see Fig. S3(a)] and we extract $\tau_{NV}$ on every z-position. For $\tau_{SiV}$, fitting the measured data with a double exponential decay is necessary [see Fig. S3(b)] because of the NV sideband PL which also partly falls in the wavelength range 735 - 745 nm. The double exponential fit reveals $\tau_{SiV}$ and $\tau_{NV}$, where the latter is consistent with the independent determination of $\tau_{NV}$ in the wavelength range 680 - 720 nm.

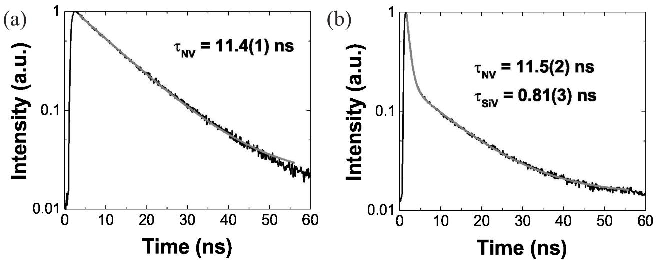


FIG. S3. Excited state lifetime measurements plotted using logarithmic scaling for the intensity for NV (a) fitted with a single exponential decay and SiV PL (b) fitted with a double exponential decay.

## VI. ODMR-SPECTRA

To determine the suitability of the tips as magnetic sensors and to prove that the tips are single crystals, we first measure ground state ODMR spectra of the embedded NV centers in a PL detection window between 680 and 720 nm. Applying a randomly-oriented magnetic field $\vec{B}$ gives us ODMR-spectra with eight dips, comparable to the measurement shown in Fig. S4. These eight dips corresponds to the four equivalent NV $\langle 111 \rangle$ orientations in the diamond lattice. The occurrence of four pairs of resonances witnesses the single crystal nature of the tip as any misoriented, polycrystalline grains would lead to additional resonances or blurring of the ODMR-spectrum. For spin manipulations, it is helpful to align the magnetic field $\vec{B}$ onto one of these NV axes and to use the sub-ensemble onto which $\vec{B}$ is aligned. This is shown in Fig. S5(a). The obtained ODMR-spectrum reveals a contrast of $C = 7.4\,\%$ [see Fig. S5(b)]. The linewidth of the dip is 12.9(5) MHz at a central frequency of 2.8 GHz. Assuming a $T_2^*$ limited linewidth, this would indicate $T_2^* \approx 13\,\mathrm{ns}$. However, Ramsey type measurement reveal $T_2^* = 0.24(7)\,\mu\mathrm{s}$, indicating significant power broadening in the ODMR spectra.

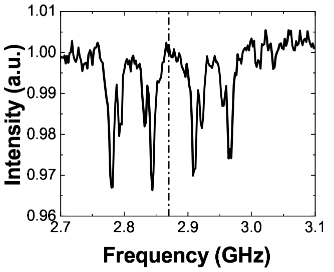


FIG. S4. Full ODMR-spectrum of the tip with randomly aligned $\vec{B}$.

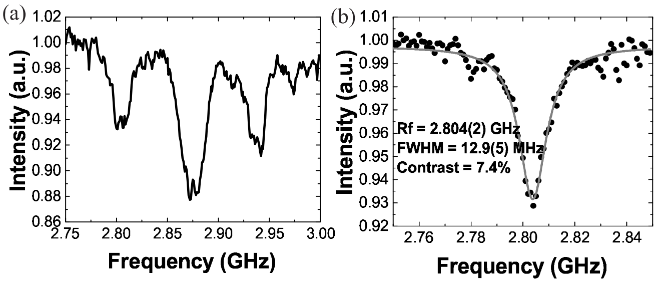


FIG. S5. (a) Full ODMR-spectrum of a tip with $\vec{B}$ aligned onto one of the NV axes. (b) Zoom onto the $m_s = 0 \to -1$ transition at a frequency of 2.8 GHz; we find a linewidth of 12.9(5) MHz. The contrast is $C = 7.4\,\%$.

As visible in Fig. S5, there is still a splitting in the central dip of 8 MHz despite the alignment onto one of the NV axes. This splitting could occur due to non-perfect alignment of the external magnetic field $\vec{B}$, because we use a permanent magnet mounted in a rotation stage on a three-axes linear translation stage. However, this splitting is also measurable when no external magnetic field is applied. Therefore, we suspect strain in the diamond itself causing this splitting.[2] However, we can not fully rule out that this splitting results from residual magnetic fields due to magnetized components in our setup which is still present after removing the magnet.

## VII. PLASMA TREATMENTS OF DIAMOND TIPS

As a first step towards optimization of the tips for magnetometry, we tested cleaning of the diamond tip using a plasma cleaning device (Diener Femto, 0.3 mbar, 4 min $O_2$ plasma with 80 W RF power at 13.56 MHz). We intended to remove possible surface contamination or highly defective regions at the tip surface. This treatment was not successful, but rather introduced additional broadband luminescence (possible due to residual contamination in the cleaning plasma), so this approach was not further investigated.
In a next step, we use an $Ar/O_2$ plasma for etching the diamond in accordance with previous approaches.[3,4] Similar plasma recipes have been found to provide highly-anisotropic etching of diamond as well as an etch rate almost independent of crystal orientation. Such a plasma can also smoothly etch polycrystalline diamond and does not selectively attack grain boundaries and defects (see Ref. 4 and the corresponding supplementary material). We use $Ar/O_2$ gases, 50 sccm each, 18.9 mTorr, 500 W ICP, 200 W RF power in an

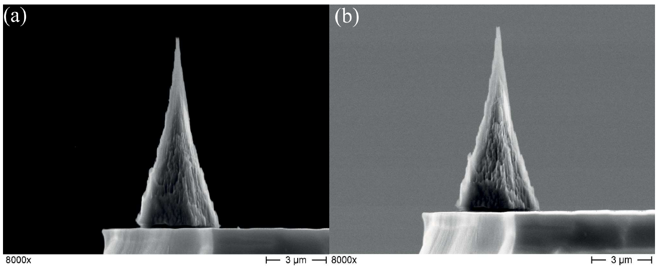


FIG. S6. 90 ° SEM picture of the tip after the second (a) and third (b) etch step.

Oxford Plasmalab inductively coupled reactive ion etcher (ICP-RIE), while the wafer is cooled to 20 °C. From etching of diamond pillars in (100) diamond using Fox16 (Dow corning) electron beam resist as mask, we determine an etch rate of ≈ 110 nm/min and verify anisotropic etching. Whereas ICP-RIE processes allow for smooth, high-rate etching of diamond and other inert materials, they simultaneously bear the risk of sample heating in the plasma. The epoxy used to mount the tip is stable up to 200 °C (information from supplier). To not exceed this temperature range, we restrict the maximum duration of the plasma steps (see below). The tip has been subjected to the following etch steps:

1. 90 s etching
2. 4 cycles of 60 s etching, 300 s cooling under Ar after each etch step
3. 3 cycles of 60 s etching, 300 s cooling under Ar after each etch step

From SEM images taken under an angle of 90° [see Fig. S6], we estimate the rate, with which the height of the pyramid is reduced during the etching to be 120 nm/min. We note that despite significant removal of diamond the surface roughness is still comparable and the pyramid still shows a sharp apex. The PL measurements reveal that we are able to significantly reduce the SiV density at the apex of the pyramid. This is shown in Fig. S7. In Fig. S7, a clear change in the spectra is visible. The SiV PL is drastically decreasing while the NV PL is nearly unchanged (compared by 3-dimensional PL maps). Thus, we are able to change the color center composition at the apex by our established plasma treatment. Please note that all these etch steps are realized while the pyramid is glued to its cantilever. Thus, we implemented a tool to tailor ready made devices.

## VIII. DISTANCE BETWEEN COLOR CENTERS

From previous work, we estimate 60 ppm silicon[5], while our measurement tentatively suggest ≈ 10 ppm nitrogen. The yield to form color centers (0.1 % for N→NV[6] and 15 % for Si→SiV[7]) indicates the parameters from Tab. I. This means that in average one out of 232 unit cells contains a NV center and one out of 28 unit cells a SiV center. This gives an approximate mean distance between centers < 10 nm at the apex. Thus, FRET between NV and SiV centers might be feasible.

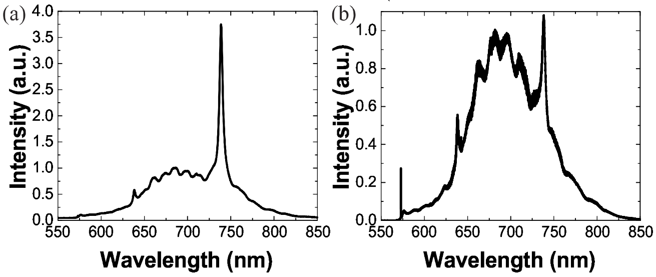


FIG. S7. PL spectra recorded at the pyramid apex before (a) and after (b) all etch steps. A significant change in SiV density is visible. This means, that we are able to actively change the color center composition at the apex of the tip. Note that the spectrum in (b) has been measured using a higher dispersion grating.

TABLE I. Parameters for the estimation of the mean distance between the color centers.

| | NV | SiV |
|---|---|---|
| Density ($cm^{-3}$/ppm) | $1.8 \cdot 10^{18}/10$ | $10^{19}/\ 57$ |
| Conversion to color center | 0.001 | 0.15 |
| Color center dens. (ppm) | 0.01 | ≈ 8 |
| number of unit cells (1D) | 232 | 28 |
| Distance between two (nm) | 83 | 10 |

[1] P. Maletinsky, S. Hong, M. S. Grinolds, B. Hausmann, M. D. Lukin, R. L. Walsworth, M. Loncar, and A. Yacoby, Nat. Nanotechnol. **7**, 320 (2012).
[2] J. Teissier, A. Barfuss, P. Appel, E. Neu, and P. Maletinsky, Phys. Rev. Lett. **113**, 020503 (2014).
[3] P. Appel, E. Neu, M. Ganzhorn, A. Barfuss, M. Batzer, M. Gratz, A. Tschöpe, and P. Maletinsky, Rev. Sci. Instrum. **87**, 063703 (2016).
[4] E. Neu, P. Appel, M. Ganzhorn, J. Miguel-Sánchez, M. Lesik, V. Mille, V. Jacques, A. Tallaire, J. Achard, and P. Maletinsky, Appl. Phys. Lett. **104**, 153108 (2014), http://dx.doi.org/10.1063/1.4871580.
[5] J. Barjon, E. Rzepka, F. Jomard, J.-M. Laroche, D. Ballutaud, T. Kociniewski, and J. Chevallier, physica status solidi (a) **202**, 2177 (2005).
[6] J. R. Rabeau, A. Stacey, A. Rabeau, S. Prawer, F. Jelezko, I. Mirza, , and J. Wrachtrup, Nano Lett. **7**, 3433 (2007).
[7] A. Bolshakov, V. Ralchenko, V. Sedov, A. Khomich, I. Vlasov, A. Khomich, N. Trofimov, V. Krivobok, S. Nikolaev, R. Khmelnitskii, and V. Saraykin, physica status solidi (a) **212**, 2525 (2015).
